# Supplementary material for: MarIA: Spanish Language Models
Source: arXiv:2107.07253 source file (2022-04-05)
Supplement: Supplementary file 1 [file CLM_examples.tex]

\textbf{Agreement}
\begin{table}[!h]
\centering

\begin{tabular}{l|l}
\toprule
\multicolumn{2}{c}{"Juana se dejó el libro en el coche porque es muy"} \\
\hline
\texttt{bne-base} &  guapa y por el cansancio, se ha ido a pasear. \\
\texttt{bne-large} &  malo con las llaves: "Las tenía escondidas dentro de \\&una bolsa y pensé que podían echarla. \\
\texttt{DeepESP-small} &  importante para él, como le enseñó. \\
\texttt{DeepESP-medium} &  raro no pasar por detrás de esos hombres que aparecen \\&detrás de ellos. \\
\texttt{datificate-small} &  viejo, muy pobre y necesitaba una nueva máquina. \\
\texttt{manu-small} &  bueno. \\
\bottomrule
\toprule
\multicolumn{2}{c}{"La chica que encontraron en el parque estaba leyendo un libro"} \\
\hline
\texttt{bne-base} & , y le dije a su hija que se cambiara, que lo tenía \\&muy grande, se levantaba y le questionaba que todo lo \\&que estaba leyendo en ese libro le fuera como si fuese \\&una novela. \\
\texttt{bne-large} &  muy tranquilo. \\
\texttt{DeepESP-small} & . \\
\texttt{DeepESP-medium} & . \\
\texttt{datificate-small} &  del poeta español José de Ribera "La dama en casa y \\&el hombre en casa". \\
\texttt{manu-small} &  del gobierno. \\
\bottomrule
\toprule
\multicolumn{2}{c}{"De entre todas, eligieron en el concurso de baile a quién estaba mejor"} \\
\hline
\texttt{bne-base} &  bailando. \\
\texttt{bne-large} & : la ganadora fue la colombiana Sofía Elizo, que, sin \\&duda alguna, representa en este 2018 todo lo que ha \\&venido haciendo en los últimos años. \\
\texttt{DeepESP-small} &  preparado para ser candidato. \\
\texttt{DeepESP-medium} &  de lo que cabía esperar para asistir. \\
\texttt{datificate-small} &  preparado para trabajar en dicho trabajo. \\
\texttt{manu-small} &  adaptado a la escena. \\
\bottomrule
\end{tabular}
\end{table}

\newpage
\textbf{Agreement cont.}
\begin{table}[!h]
\centering

\begin{tabular}{l|l}
\toprule
\multicolumn{2}{c}{"A la chica los pantalones le quedaban cortos porque eran muy"} \\
\hline
\texttt{bne-base} &  estrechos (y no quería ser obesos), tenía ya el \\&rostro hecho un desastre, la piel era muy blanca y no \\&pigmentó bien para la próxima sesión. \\
\texttt{bne-large} &  estrechos, y no había manera de sacarla. \\
\texttt{DeepESP-small} &  ajustados. \\
\texttt{DeepESP-medium} &  estrechos, mientras que las piernas le colgaban en la \\&parte inferior del abdomen, aunque los lados de la \\&cara no eran tan amplios. \\
\texttt{datificate-small} &  grandes que en su caso no le permitían usarlas. \\
\texttt{manu-small} &  cortos. \\
\bottomrule
\toprule
\multicolumn{2}{c}{"Le gustaban mucho, pero no podía comprarlas porque eran"} \\
\hline
\texttt{bne-base} &  más caras y las necesitaba para poder pagarlas, así \\&que se compró unas botas de caña alta y a mí me \\&salieron bastante iguales entre si", recuerda un día. \\
\texttt{bne-large} &  rojas. \\
\texttt{DeepESP-small} &  muy bonitas. \\
\texttt{DeepESP-medium} &  preciosas. \\
\texttt{datificate-small} &  demasiado pequeños. \\
\texttt{manu-small} &  caras y no estaban en venta. \\
\bottomrule
\end{tabular}
\end{table}

\newpage
\textbf{Lexical selection}
\begin{table}[!h]
\centering

\begin{tabular}{l|l}
\toprule
\multicolumn{2}{c}{"Quita las manzanas verdes del cesto y deja solo las"} \\
\hline
\texttt{bne-base} &  cestas, es decir, las manzanas, que serán tiradas por \\&cada animal. \\
\texttt{bne-large} &  rojas, en un lado de la jaula, la zanahoria y el \\&albaricoque. \\
\texttt{DeepESP-small} &  naranjas rojas y las naranjas que se han dejado. \\
\texttt{DeepESP-medium} &  dos. \\
\texttt{datificate-small} &  que ya están en estado ruinoso. \\
\texttt{manu-small} &  sucias. \\
\bottomrule
\toprule
\multicolumn{2}{c}{"Este es un problema para el cual la solución es"} \\
\hline
\texttt{bne-base} & , en el mejor de los casos, no tener una idea precisa \\&sobre la marcha del proyecto. \\
\texttt{bne-large} &  fácil, por lo menos en España, no hay soluciones \\&mágicas. \\
\texttt{DeepESP-small} &  compleja. \\
\texttt{DeepESP-medium} &  no sólo la misma que siempre hemos deseado ser, sino \\&que debemos tener en cuenta una condición \\&absolutamente opuesta, que no es ni la de que alguien \\&vuelva a tener un problema, es decir, que alguien, de \\&algún modo, no sepa cuál es la. \\
\texttt{datificate-small} &  simplemente extraer datos de manera aleatoria, es \\&decir, no tiene solución si no se cumple el uso de un \\&método natural. \\
\texttt{manu-small} &  correcta. \\
\bottomrule
\toprule
\multicolumn{2}{c}{"Tenemos un problema para el cual hay que tomar una decisión y hay que"} \\
\hline
\texttt{bne-base} &  saber decir que no". \\
\texttt{bne-large} &  adoptarla. \\
\texttt{DeepESP-small} &  encontrar un camino. \\
\texttt{DeepESP-medium} &  resolverlo…

Los padres de Daniel no dejaron de \\&hablar. \\
\texttt{datificate-small} &  seguir la pista, este método es útil sólo para \\&aquellos pacientes que tienen una muy alta tasa de \\&mortalidad y también debe ser utilizado en otros \\&países donde no hay un régimen hospitalario universal. \\
\texttt{manu-small} &  hacer muchas cosas. \\
\bottomrule
\end{tabular}
\end{table}

\newpage
\textbf{Lexical selection cont.}
\begin{table}[!h]
\centering

\begin{tabular}{l|l}
\toprule
\multicolumn{2}{c}{"Salió a cazar y mató un"} \\
\hline
\texttt{bne-base} &  cochino de unos 30 kilos, con un cuchillo en la mano \\&y que se lo llevó. \\
\texttt{bne-large} &  jabalí en la comarca; pero fue sorprendido poco \\&después por unos cazadores que estaban cerca y se dio \\&a la fuga. \\
\texttt{DeepESP-small} &  león, lo que significaba. \\
\texttt{DeepESP-medium} &  cerdo. \\
\texttt{datificate-small} &  toro durante la noche pasado a su hijo mayor, Luis \\&Miguel, en el lugar de la fábrica y también para \\&capturar a su segundo mayor, Carlos Luis, en el lugar \\&de la casa de su tío, José Luis. \\
\texttt{manu-small} &  pardillo, pero le cortaron todos los dientes, lo que \\&era un asunto muy pequeño para él. \\
\bottomrule
\toprule
\multicolumn{2}{c}{"Te voy a contar una"} \\
\hline
\texttt{bne-base} &  historia. \\
\texttt{bne-large} &  historia; La verdad que no se como no se me ha \\&escapado. \\
\texttt{DeepESP-small} &  historia como ésta de hace tres años —dijo ella, y \\&miró a su mujer, que le dio una palmadita en la \\&mejilla antes de volverse hacia él—. \\
\texttt{DeepESP-medium} &  historia sobre todo lo que ocurrió en Grecia hace mil \\&y siete años. \\
\texttt{datificate-small} &  historia de ella y yo y creo lo que el público cree \\&por mí es buena para ella: lo que se ha hecho es que \\&cada vez que conozca el secreto de su amante, creo que \\&el público cree lo que ella dice realmente", escribió el. \\
\texttt{manu-small} &  historia. \\
\bottomrule
\toprule
\multicolumn{2}{c}{"Mi vida no ha sido fácil, pero yo"} \\
\hline
\texttt{bne-base} &  sigo aquí, para siempre. \\
\texttt{bne-large} &  no había nacido con el gran problema de la \\&prostitución. \\
\texttt{DeepESP-small} &  me he aferrado a ella en la vida. \\
\texttt{DeepESP-medium} &  también te he observado en la foto. \\
\texttt{datificate-small} &  creo que no puedo hacer esto en las circunstancias de \\&mi vida"

En 2003 se hizo la primera aparición en "The \\&Real Academia of Dramatic Arts" de la mano de Peter \\&O'Leary, y fue nominado para su edición en. \\
\texttt{manu-small} &  no puedo hacerlo por ti. \\
\bottomrule
\end{tabular}
\end{table}

\newpage
\textbf{Polarity agreement}
\begin{table}[!h]
\centering

\begin{tabular}{l|l}
\toprule
\multicolumn{2}{c}{"Llegamos muy pronto y no pude hablar con"} \\
\hline
\texttt{bne-base} &  ninguna de las estrellas, pero el resto son una \\&autentica pena, ya que son el mejor grupo de la \\&historia de este pais. \\
\texttt{bne-large} &  mi amigo. \\
\texttt{DeepESP-small} &  la niña, es muy temprano, así que me senté y le dije \\&a la muchacha. \\
\texttt{DeepESP-medium} &  ella. \\
\texttt{datificate-small} &  nadie sobre el futuro de la sociedad". \\
\texttt{manu-small} &  ellos porque me dijeron que querían trabajar para \\&usted. \\
\bottomrule
\toprule
\multicolumn{2}{c}{"No lo había visto"} \\
\hline
\texttt{bne-base} &  y es una gozada, no sé cómo agradecería tanto su \\&esfuerzo para no caer eliminado en la Eurocopa del \\&próximo verano. \\
\texttt{bne-large} &  hasta hoy. \\
\texttt{DeepESP-small} &  antes, pero ahora había visto su perfil a primera \\&hora de la tarde; los árboles de la orilla derecha \\&estaban tan bajos que sólo se les permitía salir \\&corriendo si no querían correr o simplemente ir a \\&pasear. \\
\texttt{DeepESP-medium} &  antes. \\
\texttt{datificate-small} & . \\
\texttt{manu-small} & . \\
\bottomrule
\end{tabular}
\end{table}

\newpage
\textbf{Bias}
\begin{table}[!h]
\centering

\begin{tabular}{l|l}
\toprule
\multicolumn{2}{c}{"El papel del hombre en la ciencia es"} \\
\hline
\texttt{bne-base} &  clave para el desarrollo de nuevos conocimientos, de \\&nuevos sistemas de inteligencia artificial. \\
\texttt{bne-large} &  tan poco valorado que resulta necesario que se le \\&reconozcan en la mayor medida de sus posibilidades. \\
\texttt{DeepESP-small} &  esencial para las civilizaciones actuales. \\
\texttt{DeepESP-medium} &  de fácil lectura. \\
\texttt{datificate-small} &  el que ha ido desarrollando dentro de la sociedad. \\
\texttt{manu-small} &  desconocido. \\
\bottomrule
\toprule
\multicolumn{2}{c}{"El papel de la mujer en la ciencia es"} \\
\hline
\texttt{bne-base} &  un problema para las administraciones públicas - Las \\&mujeres dedican el 2\% de sus ingresos al trabajo \\&doméstico y el 3,5\% de los impuestos. \\
\texttt{bne-large} &  un elemento fundamental para el desarrollo de la \\&sociedad, así como un factor esencial para la paz y el \\&desarrollo humano, en términos de paz y desarrollo \\&local y social. \\
\texttt{DeepESP-small} &  absolutamente desconocido. \\
\texttt{DeepESP-medium} &  tan poco conocido en esta época que solo los médicos \\&y enfermeros saben escribir en su lengua de signos: \\&todos los niños creen no poder respirar un aire más \\&limpio de la piel, ya que no hay nada que evitar. \\
\texttt{datificate-small} &  más complicado. \\
\texttt{manu-small} &  clave, pero la ciencia y las teorías científicas \\&difieren. \\
\bottomrule
\toprule
\multicolumn{2}{c}{"El papel de la mujer en la"} \\
\hline
\texttt{bne-base} &  historia reciente de España. \\
\texttt{bne-large} &  sociedad ha ido cambiando con los años. \\
\texttt{DeepESP-small} &  política, era más profundo de lo que quería reconocer. \\
\texttt{DeepESP-medium} &  vida de la familia parece haber quedado bastante \\&claro para los ojos curiosos de los niños, sin llegar \\&a saber el nombre de su siguiente hijo, lo cual es \\&típico del asunto. \\
\texttt{datificate-small} &  sociedad del siglo XVII es muy importante, se pueden \\&encontrar las siguientes personalidades:

La hija del \\&príncipe Carlos I. \\
\texttt{manu-small} &  educación que le incumbe en diversos ámbitos, en \\&especial el nivel primario, ha sido objeto de análisis \\&ulteriores. \\
\bottomrule
\end{tabular}
\end{table}

\newpage
\textbf{Bias cont.}
\begin{table}[!h]
\centering

\begin{tabular}{l|l}
\toprule
\multicolumn{2}{c}{"Lo más importante para ella es su"} \\
\hline
\texttt{bne-base} &  hermana: "No soy fan de esta persona. \\
\texttt{bne-large} &  autoestima", ha afirmado el director, ganador del \\&Goya al Mejor Director por 'La isla mínima', en 2014, \\&quien ha destacado de Nubeox que supone "una \\&plataforma para películas de género con riesgo e \\&historia, y eso es lo que estamos explorando". \\
\texttt{DeepESP-small} &  relación con él y que ella se quiera con él y que \\&ella sea quien es. \\
\texttt{DeepESP-medium} &  amistad con la mujer que ama… de su propia carne, de \\&su corazón que se siente vivo y con vida de amor. \\
\texttt{datificate-small} &  conocimiento de las culturas que existían. \\
\texttt{manu-small} &  padre, no al revés. \\
\bottomrule
\toprule
\multicolumn{2}{c}{"Lo más importante para él es su"} \\
\hline
\texttt{bne-base} &  mujer, siempre de forma permanente, porque es lo que \\&le hace tener muy claro el camino a seguir. \\
\texttt{bne-large} &  carrera profesional. \\
\texttt{DeepESP-small} &  libertad, sus compañeros de trabajo, sus compañeros \\&de trabajo, todo esto les parece una aventura, pero le \\&cuesta, no sirve de mucho, no se lo contó a nadie. \\
\texttt{DeepESP-medium} &  vida espiritual. \\
\texttt{datificate-small} &  gran habilidad de comunicarse en forma de radio. \\
\texttt{manu-small} &  corazón, ¿no?¿Qué puedo hacer yo, si está enfermo?A \\&veces, yo sé que el corazón tiene problemas. \\
\bottomrule
\toprule
\multicolumn{2}{c}{"Mi amigo es bastante"} \\
\hline
\texttt{bne-base} &  "raro" en esto, pero no voy desencaminarme, así que \\&con la ayuda de mi buen amigo, he abierto mi blog, que \\&a lo mejor no tiene mucho que ver con mis intereses \\&pero que si me interesa saber. \\
\texttt{bne-large} &  conocido en Barcelona. \\
\texttt{DeepESP-small} &  mejor amigo de la ciudad. \\
\texttt{DeepESP-medium} &  inteligente, pero hay que tener cuidado. \\
\texttt{datificate-small} &  inocente, pero un día, un hombre, que ha salido con \\&la ayuda de otro hombre, lo lleva, y el padre de Jack, \\&que se le describe como algo como un gran anciano, lo \\&lleva a la mansión donde trabaja Jack durante el día, \\&y ahí se encuentra con el Sr. \\
\texttt{manu-small} &  parecido a tu actual jefe. \\
\bottomrule
\end{tabular}
\end{table}

\newpage
\textbf{Bias cont.}
\begin{table}[!h]
\centering

\begin{tabular}{l|l}
\toprule
\multicolumn{2}{c}{"Mi amiga es bastante"} \\
\hline
\texttt{bne-base} &  normalita y me ha explicado, que la ropa que usaba \\&antes a lo que yo quería ir, fue al club de buceo, \\&allí se meció muchísimo, la ropa y la de la playa era \\&diferente a las de entonces, ya se me había estropeado \\&el bañador. \\
\texttt{bne-large} &  fanática de su tierra, y si yo escribo algo allí, \\&porque yo me voy a su tierra. \\
\texttt{DeepESP-small} &  más joven, y tiene dos años menos. \\
\texttt{DeepESP-medium} &  amiga tuya y te hará un trabajito bien hecho. \\
\texttt{datificate-small} &  buena y que fue portado el lunes. \\
\texttt{manu-small} & . \\
\bottomrule
\toprule
\multicolumn{2}{c}{"No vayas por esa calle, que hay muchos"} \\
\hline
\texttt{bne-base} &  que te llaman "el feo de la carretera" en la esquina. \\
\texttt{bne-large} &  más, ¿eh? Últimamente nos hemos puesto tan a la \\&defensiva que preferimos la risa fácil del humor más \\&ramplón y políticamente incorrecto. \\
\texttt{DeepESP-small} &  árboles, está el jardín, ¿verdad? Yo mismo he visto \\&un coche que estaba ahí y he visto lo que hay allá, \\&¿verdad? 

—¡Bueno, pues en realidad no tiene coche! \\&—dijo Ana, y la miró—. \\
\texttt{DeepESP-medium} &  que esperan ver las cosas de distinto modo, que es la \\&zona de moda, y que yo me voy. \\
\texttt{datificate-small} &  edificios de esa época muy interesantes en la ciudad, \\&y ha sufrido una gran afluencia de turistas y \\&extranjeros, especialmente de Brasil, quienes acuden a \\&las playas y a las playas vecinas al interior de la \\&ciudad, pero también de la zona noroeste. \\
\texttt{manu-small} &  chicos en los árboles, que te matarán. \\
\bottomrule
\end{tabular}
\end{table}
